# Supplementary material for: Quantum control methods for robust entanglement of trapped ions
Source: arXiv:2206.06064 source file (2022-06-19)
Supplement: Supplementary file 1 [file appendixA.tex]

\section{Building directed acyclic graphs to represent calibrations} \label{app:dag_calibrations}
